# Supplementary material for: VesNet: Neural network accelerated solver for simulating Stokesian vesicle suspensions
Source: arXiv:2606.25569 source file (2026-06-24)
Supplement: Supplementary file 1 [file appendix_algos.tex]

Here, we summarize one time step of Ves-Net for multiple vesicles. The input consists of the configurations of $M$ vesicles, $\XX$, discretized with $N$ points, the material parameters $\kappa_b$ and $\mu$, the background velocity $\uback$ and the time step size $\Delta t$. The main algorithms are presented below: time stepping, computing tension, solving the advection problem and computing the near-singular integrals with neural networks. We refer the reader to \citet{kabacaoglu-biros19pre} for the details of the (de-)standardization algorithms. 

\begin{algorithm}[!htb]
	\caption{Ves-Net: Time stepping scheme for multiple vesicles} 
        \label{alg:time_step}
	\begin{algorithmic}
            \STATE{Given $\XX^n$ and $\sigma^n$}
            \STATE $\ubar^n = \mathtt{ComputeSingleLayerIntegral} (\XX^n, \sigma^n) + \uback(\XX^n)$ // \ref{alg:singlelayer}
            % \Comment{Velocity on vesicles}
            \STATE $\XX^* = \mathtt{SolveAdvection}(\XX^n,\ubar^n)$ \ref{alg:advect}
            % \Comment{Solving \ref{eq:advection_disc}}
            \STATE $\XX^{n+1} = \mathtt{ApproximateX_{\XX}}(\XX^*)$ 
            % \Comment{Solving \ref{eq:relaxation_disc} }
            \STATE $\sigma^{n+1} = \mathtt{ComputeTension}(\XX^{n+1}, \ubar^n)$ // \ref{alg:tension}
            % \Comment{Solving for tension \ref{eq:tension_disc}}
            \STATE $\XX^{n+1} = \mathtt{ApplyCorrectionAlgorithms}(\XX^{n+1},\mathtt{area},\mathtt{length})$
            % \Comment{See \rm{\cite{kabacaoglu-biros-e18}}}
            \RETURN $\XX^{n+1}$ and $\sigma^{n+1}$
	\end{algorithmic} 
\end{algorithm}

\begin{algorithm}[!htb]
	\caption{$\mathtt{ComputeTension}$} 
        \label{alg:tension}
	\begin{algorithmic}[1]
        \STATE // Given $\XX$ and velocity induced on the vesicle $\uu$
        \STATE $(\XX^o, \tau, \theta, \mathtt{order}) = \mathtt{standardize}(\XX)$
        % \Comment{Standardize vesicle}
        \STATE // Here, the standardization parameters are found, translation $\tau$ to center, rotation $\theta$ to align, and point ordering
        \STATE $\sigma_{\mathrm{int}}^o = \mathtt{ApproximateS_{\sigma}}(\XX^o)$
        % \Comment{Predict the map $S_{\sigma}$}
        \STATE $\uu^o = \mathtt{rotateAndOrder}(\uu,\theta,\mathtt{order})$
        % \Comment{Standardize velocity (only rotating vectors and ordering points)}
        \STATE $\{\widehat{\uu}^o_k \}_{k = 1}^{N_f} = \mathtt{fft}(\uu^o)$
        % \Comment{Compute Fourier coefficients of $\uu^o$}
        \STATE $\{ V_k \}_{k = 1}^{N_f} = \mathtt{ApproximateS_{\uu}^k}(\XX^o)$
        % \Comment{Predict the mapping $S_{\uu}^k$ to find extrinsic tension}
        \STATE $\sigma_{\mathrm{ext}}^o = \sum_k^{N_f} V_k \widehat{\uu}^o_k$
        % \Comment{Reconstruct the standardized form of the extrinsic tension term}
        \STATE $\sigma^o = \sigma_{\mathrm{int}}^o + \sigma_{\mathrm{ext}}^o$
        \STATE $\sigma = \mathtt{orderBack}(\sigma^o,\mathtt{order})$
        % \Comment{Destandardize tension by reordering points}
        \RETURN $\sigma$.
	\end{algorithmic} 
\end{algorithm}

\begin{algorithm}[!htb]
	\caption{$\mathtt{SolveAdvection}$} 
        \label{alg:advect}
	\begin{algorithmic}[1]
        \STATE // Given $\XX$ and velocity induced on the vesicle $\uu$
        \STATE $(\XX^o, \tau, \theta, \mathtt{order}) = \mathtt{standardize}(\XX)$
        % \Comment{Standardize vesicle}
        \STATE $\uu^o = \mathtt{rotateAndOrder}(\uu, \theta, \mathtt{order})$
        % \Comment{Rotate velocity and order points to standardize $\uu$}
        \STATE $\{ \widehat{\uu}_k^o\}_{k=1}^{N_f} = \mathtt{fft}(\uu^o)$
        % \Comment{Compute Fourier coefficients of $\uu^o$}
        \STATE $\{V_k \}_{k=1}^{N_f} = \mathtt{ApproximateX_{\uu}^k}(\XX^o)$
        % \Comment{Predict the action of $(1-\calM)$ on Fourier basis}
        \STATE $(1-\calM^o)\uu^o = \sum_{k}^{N_f} V_k \uu^o_k$
        % \Comment{Construct the advection part in the standardized setting}
        \STATE $\XX^{*,o} = \XX^o + \Delta t(1-\calM^o)\uu^o$
        % \Comment{Update the vesicle in the standardized setting}
        \STATE $\XX^* = \mathtt{destandardize}(\XX^{*,o},\tau,\theta,\mathtt{order})$
        % \Comment{Take back translation, rotation, and ordering}
        \RETURN $\XX^{*}$
	\end{algorithmic} 
\end{algorithm}

\begin{algorithm}[!htb]
	\caption{$\mathtt{ComputeSingleLayerIntegral}$} 
        \label{alg:singlelayer}
	\begin{algorithmic}[1]
		\STATE // Given $\XX$ and their membrane forces $\ff$ 
            \STATE Initialize $\uu_{\mathrm{near}} = 0$
            \STATE $\uu_{\mathrm{far}} = \mathtt{DirectSingleLayerIntegral}(\XX, \ff)$
             
            \STATE $\XX_q = \mathtt{FindNearFieldPoints}(\XX)$
             
            \IF{There is any $\XX_q$}
            \STATE $(\XX^o, \tau, \theta, \mathtt{order}) = \mathtt{standardize}(\XX)$
            \STATE $\xx^o_{\mathrm{layers}} = \mathtt{CreateNearLayers}(\XX^o)$
            % \Comment{Create the layers in the near-field (Fig. \ref{Fig1}) in the standardized setting}
            \STATE $\{V_k\}_{k=1}^{N_f} = \mathtt{ApproximateN_{\XX}^k}(\XX^o)$
            % \Comment{Predict the action of the single layer integral}
            \STATE $\ff^o = \mathtt{rotateAndOrder}(\ff,\theta,\mathtt{order})$
            % \Comment{Standardize the membrane force $\ff$}
            \STATE $\{ \widehat{\ff}_k\} = \mathtt{fft}(\ff^o)$
            % \Comment{Compute the Fourier coefficients of $\ff^o$}
            \STATE $\uu_{\mathrm{layers}}^o = \sum_k^{N_f} V_k \widehat{\ff}_k$
            % \Comment{Reconstruct velocity on the layers}
            \STATE $\xx_{\mathrm{layers}} = \mathtt{destandardize}(\xx_{\mathrm{layers}}^o, \tau, \theta, \mathtt{order})$
            % \Comment{Destandardize layers}
            \STATE $\uu_{\mathrm{layers}} = \mathtt{rotateAndOrderBack}(\uu_{\mathrm{layers}}^o,\theta,\mathtt{order})$
            % \Comment{Destandardize velocity on layers}
            \STATE $\uu_{\mathrm{near}} = \mathtt{interpolateInNearField}(\xx_{\mathrm{layers}},\uu_{\mathrm{layers}}, \XX_q)$
            % \Comment{Interpolate velocity on the layers for near-field}
            \ENDIF
        \STATE $\uu = \uu_{\mathrm{far}} + \uu_{\mathrm{near}}$
        \RETURN $\uu$      
	\end{algorithmic} 
\end{algorithm}
